# Supplementary material for: Influence Dynamics Among Narratives: A Case Study of the Venezuelan Presidential Crisis
Source: arXiv:2111.10402 source file (2021-11-06)
Supplement: Supplementary file 2 [file Appendices.tex]

%%%%%%%%%%%%%%%%%%%%%%%%%%%%%%%%%%%%%%%%%%%%%%%%%%%%%%%%%%%%%%%%%%%%%%%%%%%%%%%%
%%%%%%%%%%%%%%%%%%%%%%%%%%%%%%%%%%%%%%%%%%%%%%%%%%%%%%%%%%%%%%%%%%%%%%%%%%%%%%%%
%%%%%%%%%%%%%%%%%%%%%%%%%%%%%%%%%%%%%%%%%%%%%%%%%%%%%%%%%%%%%%%%%%%%%%%%%%%%%%%%
\section{\OURMEASURE-related results (Akshay)}

\begin{itemize}

	\item time frame \#1 (December 25, 2018 to December 26, 2018):
	\begin{itemize}
		\item \textit{const} significantly influences \textit{assembly}.
		\item \textit{crisis} significantly influences \textit{protests}.
		\item \textit{other/anti\_socialism} strongly influences \textit{guaido/legitimate}.
	\end{itemize}

	\item time frame \#2 (December 26, 2018 to December 27, 2018):
	\begin{itemize}
		\item \textit{guaido/legitimate} strongly influences \textit{assembly}.
		\item \textit{maduro/legitimate} weakly influences \textit{guaido/legitimate}.
		\item \textit{protests} significantly influences \textit{assembly}.
		\item \textit{other/anti\_socialism} significantly influences \textit{guaido/legitimate}.
	\end{itemize}

	\item time frame \#3 (December 27, 2018 to December 28, 2018):
	\begin{itemize}
		\item \textit{guaido/legitimate} weakly influences \textit{assembly}.
		\item \textit{protests} significantly influences \textit{assembly}.
	\end{itemize}

	\item time frame \#4 (December 28, 2018 to December 29, 2018):
	\begin{itemize}
		\item \textit{guaido/legitimate} significantly influences \textit{assembly}.
		\item \textit{protests} strongly influences \textit{assembly}.
	\end{itemize}

	\item time frame \#5 (December 30, 2018 to December 31, 2018):
	\begin{itemize}
		\item \textit{military} significantly influences \textit{crisis}.
		\item \textit{assembly} weakly influences \textit{guaido/legitimate}.
		\item \textit{maduro/legitimate} weakly influences \textit{assembly}.
		\item \textit{arrests} weakly influences \textit{guaido/legitimate}.
		\item \textit{arrests} significantly influences \textit{crisis}.
	\end{itemize}

	\item time frame \#6 (December 31, 2018 to January 01, 2019):
	\begin{itemize}
		\item \textit{military} weakly influences \textit{assembly}.
		\item \textit{guaido/legitimate} significantly influences \textit{crisis}.
		\item \textit{protests} weakly influences \textit{assembly}.
		\item \textit{other/anti\_socialism} weakly influences \textit{crisis}.
	\end{itemize}

	\item time frame \#7 (January 01, 2019 to January 02, 2019):
	\begin{itemize}
		\item \textit{const} strongly influences \textit{other/anti\_socialism}.
		\item \textit{protests} significantly influences \textit{other/anti\_socialism}.
		\item \textit{arrests} significantly influences \textit{assembly}.
	\end{itemize}

	\item time frame \#8 (January 02, 2019 to January 03, 2019):
	\begin{itemize}
		\item \textit{arrests} significantly influences \textit{assembly}.
	\end{itemize}

	\item time frame \#10 (January 04, 2019 to January 05, 2019):
	\begin{itemize}
		\item \textit{arrests} significantly influences \textit{crisis}.
	\end{itemize}

	\item time frame \#17 (January 11, 2019 to January 12, 2019):
	\begin{itemize}
		\item \textit{maduro/legitimate} significantly influences \textit{military}.
	\end{itemize}

	\item time frame \#18 (January 12, 2019 to January 13, 2019):
	\begin{itemize}
		\item \textit{military} weakly influences \textit{guaido/legitimate}.
		\item \textit{maduro/legitimate} strongly influences \textit{guaido/legitimate}.
	\end{itemize}

	\item time frame \#20 (January 14, 2019 to January 15, 2019):
	\begin{itemize}
		\item \textit{arrests} decisively influences \textit{protests}.
	\end{itemize}

	\item time frame \#22 (January 16, 2019 to January 17, 2019):
	\begin{itemize}
		\item \textit{maduro/legitimate} significantly influences \textit{arrests}.
	\end{itemize}

	\item time frame \#23 (January 17, 2019 to January 18, 2019):
	\begin{itemize}
		\item \textit{maduro/legitimate} weakly influences \textit{arrests}.
	\end{itemize}

	\item time frame \#25 (January 19, 2019 to January 20, 2019):
	\begin{itemize}
		\item \textit{assembly} weakly influences \textit{arrests}.
		\item \textit{other/anti\_socialism} strongly influences \textit{arrests}.
	\end{itemize}

	\item time frame \#26 (January 20, 2019 to January 21, 2019):
	\begin{itemize}
		\item \textit{military} significantly influences \textit{protests}.
	\end{itemize}

	\item time frame \#28 (January 22, 2019 to January 23, 2019):
	\begin{itemize}
		\item \textit{maduro/legitimate} strongly influences \textit{other/anti\_socialism}.
	\end{itemize}

	\item time frame \#30 (January 24, 2019 to January 25, 2019):
	\begin{itemize}
		\item \textit{other/anti\_socialism} significantly influences \textit{military}.
	\end{itemize}

	\item time frame \#32 (January 26, 2019 to January 27, 2019):
	\begin{itemize}
		\item \textit{military} weakly influences \textit{other/anti\_socialism}.
	\end{itemize}

	\item time frame \#33 (January 27, 2019 to January 28, 2019):
	\begin{itemize}
		\item \textit{crisis} weakly influences \textit{guaido/legitimate}.
	\end{itemize}

\end{itemize}

\textbf{Observations:}
\begin{itemize}
    
    \item In 15 (out of 35; $\sim43\%$) time frames, all narratives are self-sustaining. Of particular note is the span of time frames \#11 through \#16 (2019-01-05 through 2019-01-11).
    
    \item \textit{assembly} gets co-influenced by \textit{protests} and \textit{guaido/legitimate} in time frames \#2, \#3 and \#4 (2018-12-26 through 2019-01-01).

    \item \textit{maduro/legitimate} never gets influenced by any other narrative.

    \item The \textit{assembly} and \textit{crisis} narratives, along with \textit{const} (other sources) appear to exert influence on other narratives very few times. 
    
\end{itemize}

%%%%%%%%%%%%%%%%%%%%%%%%%%%%%%%%%%%%%%%%%%%%%%%%%%%%%%%%%%%%%%%%%%%%%%%%%%%%%%%%
%%%%%%%%%%%%%%%%%%%%%%%%%%%%%%%%%%%%%%%%%%%%%%%%%%%%%%%%%%%%%%%%%%%%%%%%%%%%%%%%
%%%%%%%%%%%%%%%%%%%%%%%%%%%%%%%%%%%%%%%%%%%%%%%%%%%%%%%%%%%%%%%%%%%%%%%%%%%%%%%%
\section{Snippets of Older Material (Remove, When Applicable)}

%%%%%%%%%%%%%%%%%%%%%%%%%%%%%%%%%%%%%%%%%%%%%%%%%%%%%%%%%%%%%%%%%%%%%%%%%%%%%%%%
%%%%%%%%%%%%%%%%%%%%%%%%%%%%%%%%%%%%%%%%%%%%%%%%%%%%%%%%%%%%%%%%%%%%%%%%%%%%%%%%
\subsection{Xixi's Self- \& Cross-Narrative Influence Characterization via \acp{MVHP} subsection}

% Akshay: here, please describe the entire experimental setup and how we used \acp{MVHP} to infer influences.

We only consider a single exogenous influence that we denote by the set \{$ {constant} $\}. This also gives us the option of considering other influences, although we leave that to future work.The ``constant'' exogenous source with constant value $1$, i.e. a step function, is used to model the base rate of the narrative event. $\alpha_{kp}$ quantifies the magnitude of the corresponding exogenous source influence to the $k$-th narrative event rate.

$\mathcal{Q}$ is the set of narratives as described in section \ref{sec:dataset}. As shown by the conditional intensity in equation \ref{eq:conditional_intensity}, each previous event, both from its own narrative(self-) and other narratives(cross-), will create a positive excitation to the $k$-th narrative event. We choose the decaying exponential function as triggering function $\phi(\tau) = \mathrm{e}^{-\tau}$ to indicate the decaying influence of  history events. Similarly, the $\alpha_{kq}$ measures the magnitude of influence from the $q$-th narrative to the $k$-th narrative.

%%%%%%%%%%%%%%%%%%%%%%%%%%%%%%%%%%%%%%%%%%%%%%%%%%%%%%%%%%%%%%%%%%%%%%%%%%%%%%%%
%%%%%%%%%%%%%%%%%%%%%%%%%%%%%%%%%%%%%%%%%%%%%%%%%%%%%%%%%%%%%%%%%%%%%%%%%%%%%%%%
\subsection{Akshay's Discussion snippet(s)}

...fitted a \ac{MVHP} per time window of 2 days between the 25\textsuperscript{th} January and 1\textsuperscript{st} of February. We here interpret the heat-maps (as shown in  \figref{fig:probability_heatmaps}) generating using the aforementioned \OURMEASURE for each narrative-narrative pair. This, as mentioned earlier, provides a semantic agnostic influence between processes by restricting the values as probabilities.  In this section, we describe some deviations of note in some specific \OURMEASURES and further explore the real world events that could have prompted them. We note that the overarching trend of \OURMEASURES across the time-periods have been one of the self-influencing nature , i.e. the most likely cause for event from a narrative is a past event from the same narrative. This, we argue, owns itself to tweets about certain narratives driving the conversation themselves and, to an extent, thriving in a bubble of their own making. 

Our findings indicate that the \ac{MVHP} provides insights into the crisis in a complementary sense. While the results we obtain do not reveal subtleties of the dynamics between the narratives, they provide a feasible way of ingesting the massive amounts of social media data and provide insights that could perhaps help confirm certain ideas postulated by political scientists. For instance, deviations of narratives from self-excitation asks of us the following questions: Do such deviations persist across or re-occur in time? What real-world event could have prompted such a deviation? Do such deviations warrant further investigations into the data? We attempted to answer these questions in a necessarily speculative fashion and mean to show how political scientists could make use of our methodology as tool to discover influences among narratives.

% ``bring latent influences to the forefront''

%%%%%%%%%%%%%%%%%%%%%%%%%%%%%%%%%%%%%%%%%%%%%%%%%%%%%%%%%%%%%%%%%%%%%%%%%%%%%%%%
%%%%%%%%%%%%%%%%%%%%%%%%%%%%%%%%%%%%%%%%%%%%%%%%%%%%%%%%%%%%%%%%%%%%%%%%%%%%%%%%
\subsection{Previous Abstract}

The diffusion of information online has overarching consequences on the sovereignty and stability of regions. Knowing how ideas spread in social media can further our understanding of the geopolitical environment in which these ideas thrive. In this work, we seek to evaluate the relationship between different narratives as they take place in Twitter during the 2019 Venezuelan Presidential Crisis. To this end, we model diffusion of information within Twitter as a stochastic temporal point process and derive influence measures that help us interpret its parameters by virtue of explainable properties of such models. We learn these models in moving time frames of 2 days throughout the duration of interest so as to capture fleeting influences. We make use of Twitter data to discern how ideas in social media messaging evolve and influence each other and establish how they relate to events having taken place in the real world. Such a tool could aid political and social scientists to complement existing knowledge about socio-political phenomena. % We conclude with a discussion of our approach and its relevance to studying genuine and manipulated information diffusion.

%%%%%%%%%%%%%%%%%%%%%%%%%%%%%%%%%%%%%%%%%%%%%%%%%%%%%%%%%%%%%%%%%%%%%%%%%%%%%%%%
%%%%%%%%%%%%%%%%%%%%%%%%%%%%%%%%%%%%%%%%%%%%%%%%%%%%%%%%%%%%%%%%%%%%%%%%%%%%%%%%
\subsection{Previous last paragraphs in Introduction}

We intend to model the continuously evolving dynamics of narratives, whose definition follows \cite{Blackburn2020CorpusDF} -- ``recurring statements that express a point of view''. In this study, we evaluate the dynamics of narratives in Twitter under the prism of causal influence among narratives. We utilise a system self- and mutually-exciting stochastic \ac{TPP}s, namely \ac{MVHP} \cite{Hawkes1971}, to model events from multiple narratives and how they influence each other. This influence is determined via moving time frames to recognize temporary influences, which, in the case of \cite{Lai2016} and \cite{Mohler2020}, would have been regarded as noise. This is especially important in the case of Venezuela with continuously evolving narratives within the time frame of interest. Furthermore, we make use of the explainability of these models to derive a set of \OURMEASURES that can complement existing knowledge about the crisis. This can provide social and political scientists with the tools necessary to better analyse social media events and perhaps help to paint a comprehensive portrait of political discourse in a country. Our findings indicate that our dynamic model responds to events of interest in the Venezuelan presidential crisis. We describe our point process model in \secref{sec:methodology}. The Twitter dataset, the data labelling strategy, and relevant definitions are discussed in \secref{sec:dataset} and, finally, \secref{sec:discussion} involves discussion of the results.

In this study, we evaluate the dynamics of narratives in Twitter under the prism of causal influence among narratives. We utilise a system self- and mutually-exciting stochastic \ac{TPP}s, namely \ac{MVHP} \cite{Hawkes1971}, to model events from multiple narratives and how they influence each other. This influence is determined via moving time frames to recognize temporary influences, which, in the case of \cite{Lai2016} and \cite{Mohler2020}, would have been regarded as noise. This is especially important in the case of Venezuela with continuously evolving narratives within the time frame of interest. Furthermore, we make use of the explainability of these models to derive a set of \OURMEASURES that can complement existing knowledge about the crisis. This can provide social and political scientists with the tools necessary to better analyse social media events and perhaps help to paint a comprehensive portrait of political discourse in a country. Our findings indicate that our dynamic model responds to events of interest in the Venezuelan presidential crisis.  The Twitter dataset, the data labelling strategy, and relevant definitions are discussed in \secref{sec:dataset}.  We describe our point process model in \secref{sec:methodology}and, finally, \secref{sec:discussion} involves discussion of the results.

%%%%%%%%%%%%%%%%%%%%%%%%%%%%%%%%%%%%%%%%%%%%%%%%%%%%%%%%%%%%%%%%%%%%%%%%%%%%%%%%
%%%%%%%%%%%%%%%%%%%%%%%%%%%%%%%%%%%%%%%%%%%%%%%%%%%%%%%%%%%%%%%%%%%%%%%%%%%%%%%%
\subsection{Previous Dataset Section}

%I think much of the text in the Table caption above should be in the body of the paper, not as a caption.  

The Twitter dataset used for this study is a subset of a larger social media dataset curated by a data provider as part of a larger grant program and is described in \cite{Blackburn2020Venezuela}. In accordance with the requirements of the organization funding the research, the data were anonymized prior to sharing it with researchers to protect privacy. Overall, it encompasses over 7 million tweets from December 25\textsuperscript{th}, 2018, to February 1\textsuperscript{st}, 2019, which marks the commencement of the presidential crisis. The tweets were annotated with labels associated with their narratives and their stances towards Maduro. We evaluated the diffusion of narratives as defined in \cite{Blackburn2020CorpusDF}. The tweets were collected using a set of keywords determined by subject matter experts (SME). % who had familiarity with the Venezuelan succession crisis. 
A subset of these tweets, which contained both English and Spanish language texts, was then manually labelled to train BERT-based Multilingual Cased model \cite{pires2019}. Additionally, as described, we also refer to stance information as described by \cite{Blackburn2020CorpusDF} to understand how each narrative tends to support or oppose Maduro. % and these are class labels that indicate a tweet being either in support or against Maduro.
% Although we do not model the dynamics of the stances, it helps provide context as to why one narrative may influence another.

\begin{figure}[htpb!]
    \centering
    \includegraphics[scale=0.2]{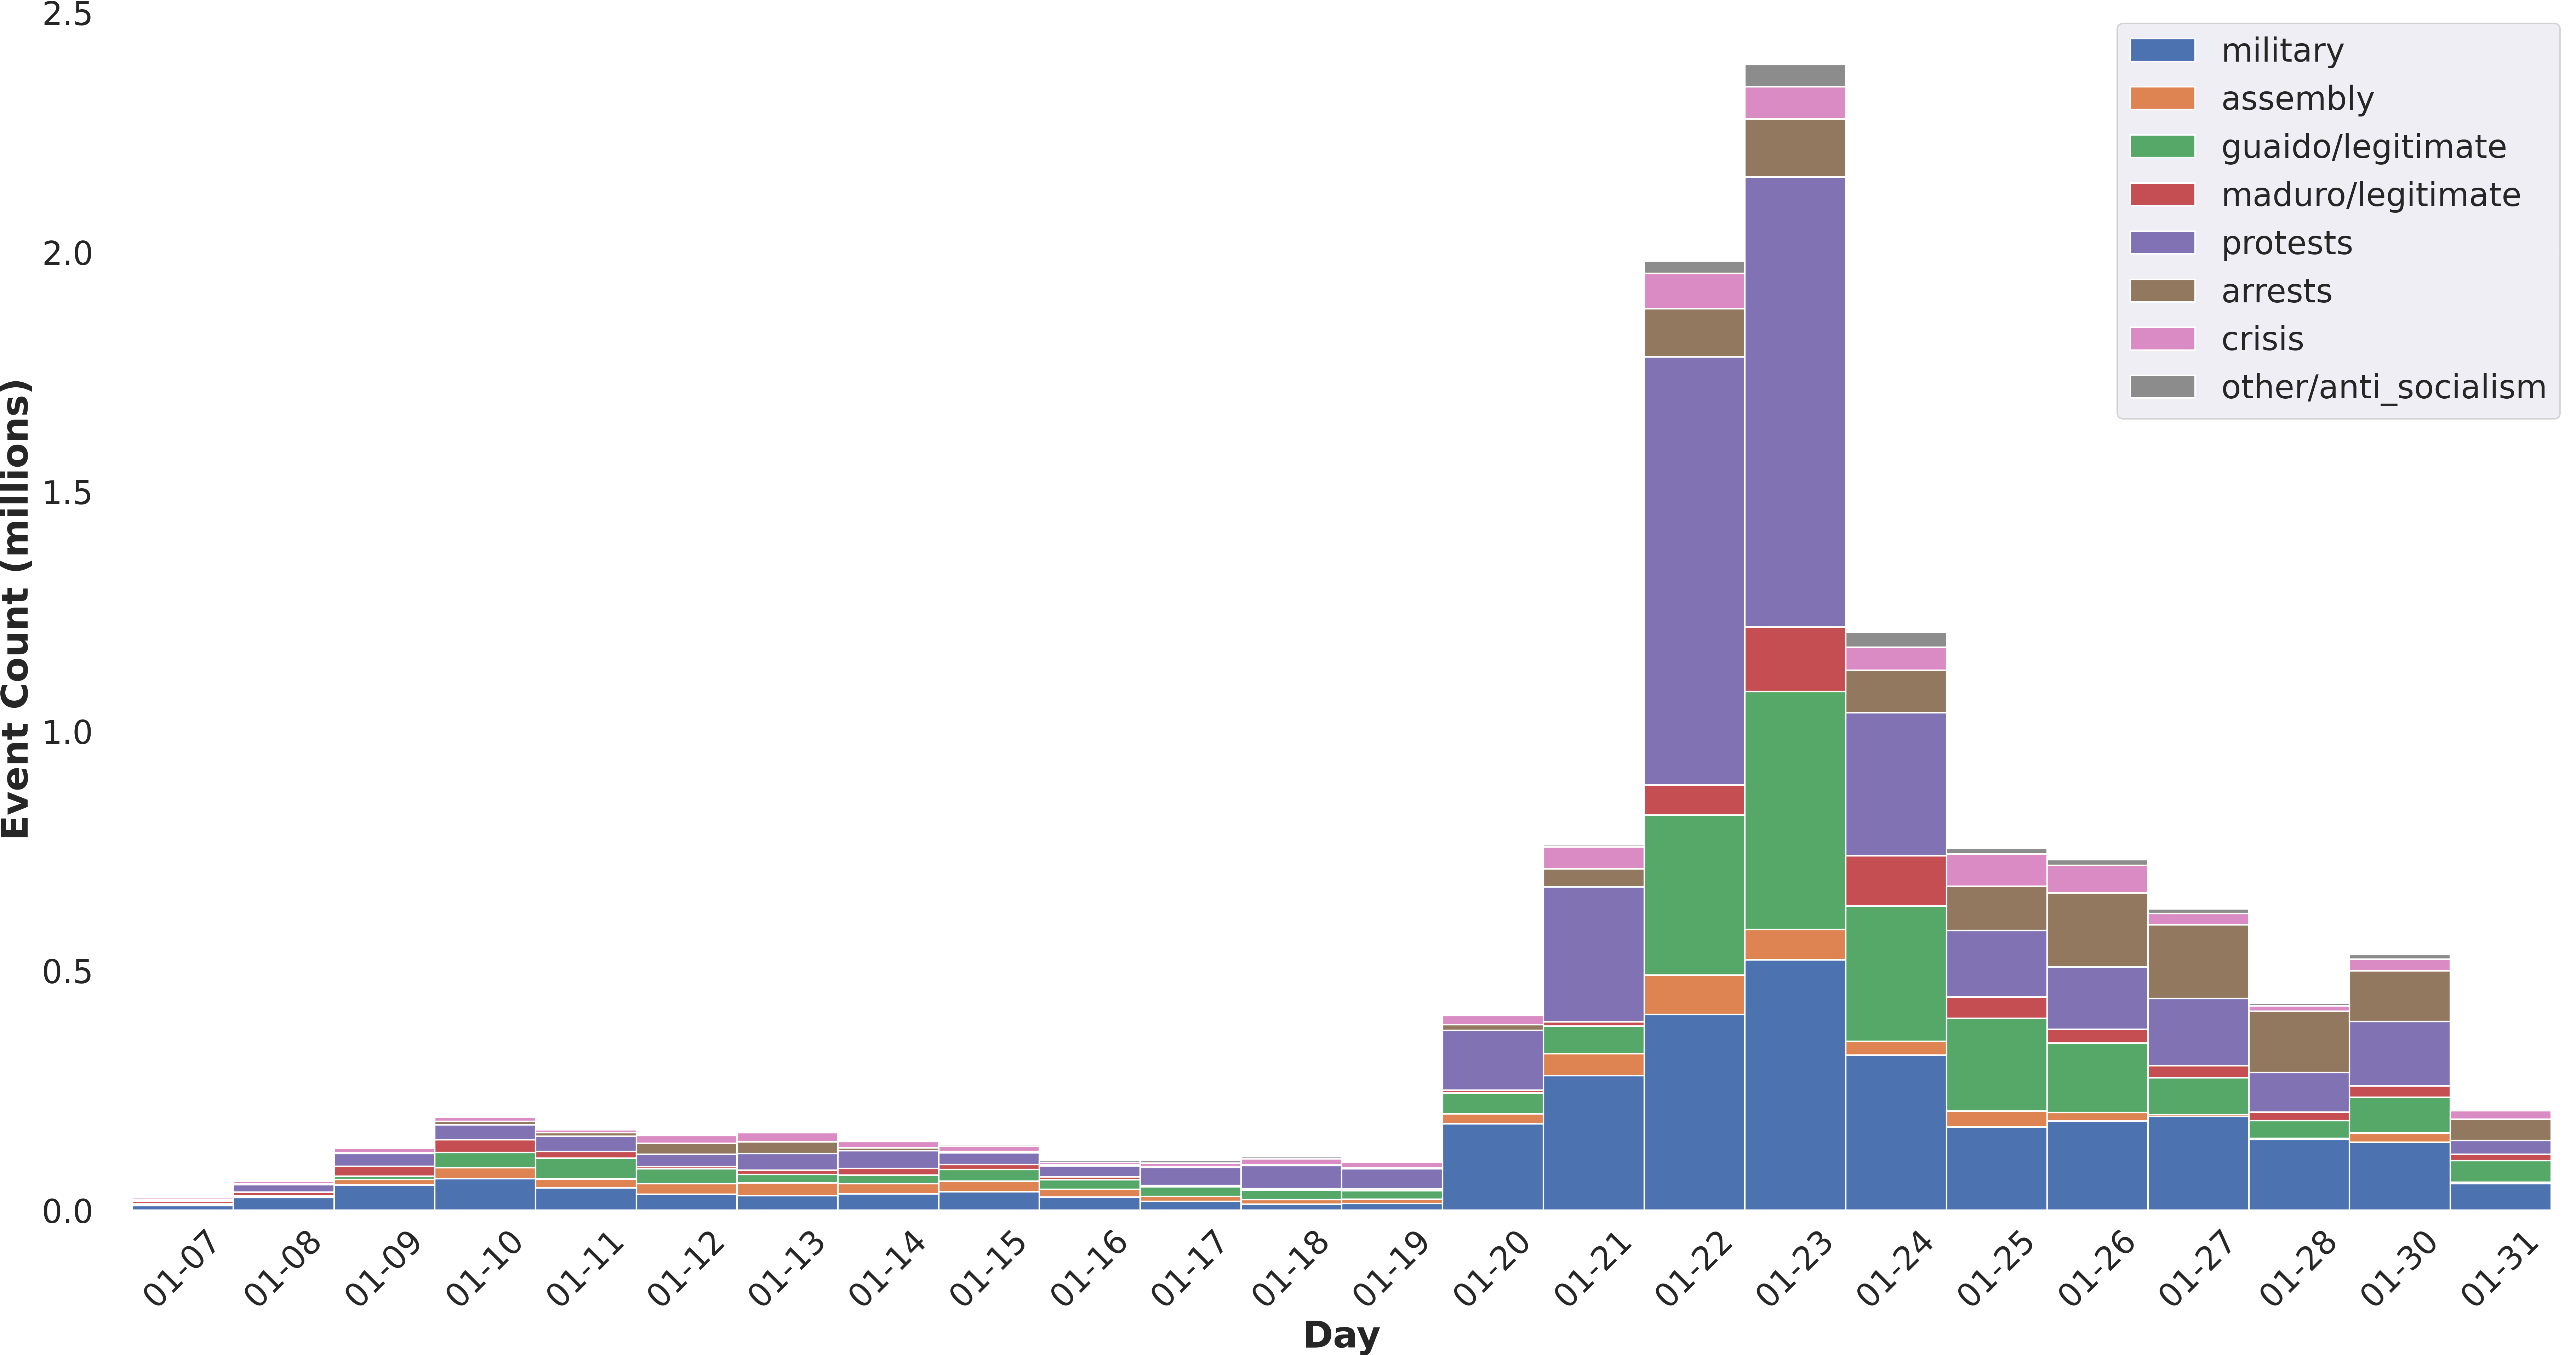}
    \caption{Histogram of Twitter event counts with contribution by individual narratives. We see a jump in events between the 20\textsuperscript{th} and 21\textsuperscript{st} of January during which there was a small-scale coup initiated by 27 soldiers. There is a bigger jump in event count on the 23\textsuperscript{rd} of January was a result of the massive protests held with the intention to force Maduro to step down, during which time period, we also witness a significant increase in anti-Maduro tweets.}
    \label{fig:event_count_histograms___}
\end{figure}

\begin{table}[htpb]
    \centering
    \begin{tabularx}{\textwidth}{@{} p{0.3\textwidth} p{0.233\textwidth} p{0.233\textwidth} p{0.233\textwidth} @{}}
        \toprule         
        \textbf{Narrative} & \textbf{Total Tweets} & \textbf{\% anti-Maduro} & \textbf{\% pro-Maduro} \\
        \midrule
        \addlinespace[5pt]
        \textit{military} & 1,534,242 & 67.38 & 21.87 \\
        \textit{assembly} & 252,448 & 95.79 & 1.82 \\
        \textit{guaido/legitimate} & 1,014,726 & 95.43 & 3.02 \\
        \textit{maduro/legitimate} & 304,127 & 2.92 & 96.72 \\
        \textit{protests} & 1,746,615 & 85.87 & 2.42 \\
        \textit{arrests} & 570,574 & 97.73 & 0.74 \\
        \textit{crisis} & 305,291 & 73.25 & 3.58 \\
        \textit{anti-socialism} & 101,716 & 78.04 & 14.77 \\
        \addlinespace[5pt]
        \bottomrule
        \addlinespace[5pt]
    \end{tabularx}
    \caption{Stance distribution per narrative of the Venezuela Twitter data.}
    \label{tab:data_description___}
\end{table}

% , including those such as FANB (national Bolivarian armed forces), DGCIM (Directorate General of Military Counterintelligence), GNB (Bolivarian national guard), and armed paramilitary groups that were loyal to Maduro such as “colectivos”.
% : \textit{military}, \textit{assembly}, \textit{guaido/legitimate},\textit{maduro/legitimate}, \textit{protests}, \textit{arrests}, \textit{crisis} and \textit{anti-socialism}

Narratives constitute tweets that express a point of view having to do with specific topics related to the Venezuelan presidential crisis \cite{Blackburn2020CorpusDF}. We note that tweets can be associated with multiple narratives, in which case, we treat each tweet separately per narrative. We only considered narratives that were present in at least 100,000 tweets. As a result, we analyzed a total of 8 narratives. \tabref{tab:data_description} shows the distribution of stances per narrative and \figref{fig:event_count_histograms} shows the distribution of narratives with event counts in the time period of interest. The \textit{military} narrative includes discussion about the Venezuelan army, security services, or other organizations that reported to Maduro's government. \textit{Assembly} includes any mentions of the National Assembly. \textit{Guaido/legitimate} and \textit{maduro/legitimate} include all tweets that expressly support or simply state a point about the legitimacy of Guaid\'{o} and Maduro, respectively. \textit{Protests} includes tweets that mention anti-Maduro demonstrations, public gatherings, or rallies. \textit{Arrests} includes tweets that refer to people who have been taken prisoner. The \textit{crisis} narrative label refers to the Venezuelan humanitarian crisis and finally, \textit{anti-socialism} includes tweets that mention socialism, communism, or leftism as the primary cause of the humanitarian crisis.
